# Supplementary material for: On the Calibration of Epistemic Uncertainty: Principles, Paradoxes and Conflictual Loss
Source: arXiv:2407.12211 source file (2024-07-16)
Supplement: Supplementary file 1 [file main.tex]

\documentclass[runningheads]{llncs}
\usepackage[T1]{fontenc}
\usepackage{graphicx}
\usepackage{booktabs}
\usepackage[misc]{ifsym}

% N.B.: do not change anything above this line. If you require additional packages, please load them directly after this line.
\usepackage{mwe}
% N.B.: you may delete the preceding line. It is used to display an example image in this template.

\usepackage[leqno]{amsmath}
\usepackage{amssymb}
\usepackage{bbm}
\usepackage{bm}
\usepackage{tikz}
\usepackage[font=scriptsize]{subcaption}
\usepackage[colorlinks=true]{hyperref}
\usepackage[title]{appendix}

\usepackage{array}
\newcolumntype{P}[1]{>{\centering\arraybackslash}p{#1}}
\usepackage{booktabs}

\begin{document}

\title{On the Calibration of Epistemic Uncertainty: Principles, Paradoxes and Conflictual Loss}
\titlerunning{On the Calibration of Epistemic Uncertainty}

\author{}
\institute{}

\maketitle

\input{annex_content}

\medskip
\bibliographystyle{splncs04}
\bibliography{biblio}

\end{document}
